# Supplementary material for: Finite time analysis of temporal difference learning with linear function approximation: Tail averaging and regularisation
Source: arXiv:2210.05918 source file (2024-09-19)
Supplement: Supplementary file 1 [file appendix-regtd.tex]

\section{Regularised TD}
    \noindent Regularised TD update: 

    \begin{align*}
        \hat\params_{\timestep+1} &= (\identity - \lr \lambda)\hat\params_{\timestep} + \lr (-A \hat\params_\timestep + b \Delta M_\timestep).
    \end{align*}
    
    \noindent Solution of for the regularised TD iteration:
    \begin{align*}
        \params^{\star}_{\mathsf{reg}} &= (A + \lambda \identity)^{-1}b.
    \end{align*}
    
    % \noindent Now define the centered update as follows:
    % \begin{align*}
    %     \hat z_{\timestep+1} &= \hat\params_{\timestep+1} - \hat\params^\star = (\identity - \lr (\lambda\identity + A))(\hat\params_\timestep - \hat\params^\star) + \lr \Delta M_\timestep,\\
    %     &= (\identity - \lr (\lambda\identity + A))\hat z_\timestep + \lr \Delta M_\timestep.\numberthis\label{eq:centered-reg-update}
    % \end{align*}
    
  \begin{lemma}\label{lem:regtd-highprob-helper1}
        Let $\lr \leq \lr_{\text{max}}$, where $\lr_{\text{max}}$ is set as per \eqref{eq:reg-td-lr}, then for any any $\hat \params$ we have the following result:
        \begin{align*}
            \expecun{}[\hat{\params}^{\top} (\identity - \lr (\lambda \identity & + a_j))\tr (\identity - \lr (\lambda \identity + a_j))\hat{\params} \vert \mathcal{F}_{j-1}] \leq (1-2\lr\mu)\norm{\hat \params}_{2}^{2},
        \end{align*}
        where $a_{j} \define [\feature(\state_{j})\feature(\state_{j}){\tr} - \discount\feature(\state_{j})\feature(\state'_{j}){\tr}]$.  
    \end{lemma}
   \begin{proof}
         \begin{align*}
            \expecun{}[\hat{\params}^{\top} (\identity - \lr (\lambda \identity & + a_j))\tr (\identity - \lr (\lambda \identity + a_j))\hat{\params} \vert \mathcal{F}_{j-1}]\\ &= \expecun{}[\hat{\params}^{\top} (\identity - 2\lr\lambda\identity - \lr(a_j + a_{j}\tr) + \lr^2\{ \lambda^2 \identity + \lambda  (a_j + a_{j}\tr) + a_{j}\tr a_j\} ) \hat{\params} \vert \mathcal{F}_{j-1}],\\
            &= \expecun{}[\hat{\params}^{\top}\hat{\params}\vert\mathcal{F}_{j-1}] -  \lr \expecun{}[\hat{\params}\tr 2\lambda \identity \hat{\params} \vert \mathcal{F}_{j-1}] -\lr \underbrace{\hat{\params}^{\top} \expecun{}[ a^{\top}_j + a_j \vert\mathcal{F}_{j-1}] \hat{\params}}_{A1} +\\ 
            &\lr^2 \underbrace{\hat{\params}^{\top}\expecun{}[ a_{j}^{\top}a_j\vert \mathcal{F}_{j-1}]\hat{\params}}_{A2} + \lr^2 \underbrace{\hat{\params}\tr\expecun{}[a_{j} + a_{j}\tr\vert \mathcal{F}_{j-1}]\hat{\params} }_{A3}+ \lr^2 \expecun{}[\hat{\params}\tr \lambda^2\identity \hat{\params} \vert \mathcal{F}_{j-1}]  .
        \end{align*}
        The bounds on terms (A1) and (A2) can be referred from \cref{eq:bound-tA1}, and \cref{eq:bound-tA2} of \Cref{lem:high-prob-helper-1}
        
       Bounding (A3):
       \begin{align*}
           \hat{\params}\tr\expecun{}[a_{j} + a_{j}\tr\vert \mathcal{F}_{j-1}]\hat{\params} &= \hat{\params}\tr (A+ A\tr) \hat{\params},\\
           &\stackrel{(a)}{\leq} (1+\discount)\hat{\params}^{\top}B\hat{\params}\\
       \end{align*}
       where $(a)$ follows from \Cref{lem:A-lower}.
       Putting everything together we get:
       \begin{align}
           \expecun{}[\hat{\params}^{\top} (\identity - \lr (\lambda \identity & + a_j))\tr (\identity - \lr (\lambda \identity + a_j))\hat{\params} \vert \mathcal{F}_{j-1}]\\
           &\leq \params\tr( 1 - \lr \left(2(1-\discount) B + 2\lambda - \lr(\lambda^{2} + (1+\discount)B + (1+\discount)^{2}\Feature_{\text{max}}^{2}B \right))\params\\
       \end{align}
       where $(a)$ follows from using the using the value of $\lr_\text{max}$ given in \eqref{eq:reg-td-lr}.
    \end{proof}
